# Supplementary material for: Data-driven and low-rank implementations of Balanced Singular Perturbation Approximation
Source: arXiv:2303.05361 source file (2023-03-09)
Supplement: Supplementary file 1 [file secAppendix.tex]

%Ideas for a future related proceeding...
%%\appendix

%%
\section{Reduction of shifted system}
[J. YANG , C. S. CHEN, et al: \textit{Model reduction of unstable systems}...,1993] propose a modified \BT (modified \SPA), in which the balancing is done w.r.t. the generalized Gramians. (Interpretation: Projection bases obtained from shifted system; projection step done on original system)

\subsection{The method relying on shifted Gramians}
Let $\xs \geq 0$. The generalized Gramians $\bP_\xs$ and $\bQ_\xs$ of the shifted system are defined as the solution of
\begin{align*}  %%\label{lyapEq}
(\bA - \xs \bI) \bP_\xs + \bP_\xs (\bA - \xs \bI)^T + \bB\bB^T = \bv{0}, \\
(\bA - \xs \bI)^T \bQ_\xs + \bQ_\xs (\bA - \xs \bI) + \bC^T \bC = \bv{0}. 
\end{align*}

Motivation 1: These Gramians are well-defined for unstable systems, when $\xs$ is chosen sufficiently large.

Motivation 2: In frequency-space applications, where only frequencies with larger real part than $\xs$ are relevant, this approach gives better results. (Note: The error also excludes all frequencies with smaller real part than $\xs$)

\subsection{Data-driven realization of the shifted methods}

The generalized Gramians have the following representation in frequency space
\begin{align} \label{gram_P_gen}
\begin{split}
\bP_\xs &=
\frac{1}{2\pi}\int_{-\infty}^{\infty} ((\imunit \zeta +\xs)\bI -\bA)^{-1} \bB \bB^T ((-\imunit \zeta+\xs)\bI^T -\bA^T)^{-1} d \zeta. \\
\bQ_\xs &= \frac{1}{2\pi}\int_{-\infty}^{\infty} ((-\imunit \omega+ \xs) \bI -\bA^T)^{-1} \bC^T \bC ((\imunit \omega+\xs)\bI -\bA)^{-1} d \omega.
\end{split}
\end{align}

Proposition~\ref{prop:quadMatrices}, which is the basis of the data-driven implementations, generalizes naturally for the shifted Gramians: Replace $\TFs$ by
$\TFs_\xs$ which is defined by $\TFs(s) = \TFs(s+\xs)$ everywhere. The only adaption required in Algorithm~\ref{alg:quadbt} and Algorithm~\ref{alg:quadspq} is that samples of this shifted transfer functions are taken.

\begin{remark}
The shifted method is not to be confused with the generalized singular perturbation approximation considered in [] %Guiver...
The cited methods consist of balancing the system, afterwards including a shift, then reduce, and then shift back. Balancing and shifting do not commute! The method proposed in this section only shifts and reduces but does no back shift.
\end{remark}

\subsection{Old stuff that became obsolete}

\begin{algorithm}[htp] 
	\caption{Quadrature-based (data-driven) Singular Perturbation Approximation (\QSPA)}  
	\label{alg:quadspq}                                     
	\algorithmicrequire~\LTI system described through a transfer function evaluation map, $\TF(s)$; \\
	%%\hspace*{5mm} Frequency shift $\xi {\color{red}\in \IR^+ }$ \\ %TODO	
	\hspace*{5mm} quadrature nodes, $\omega_j$, and weights, $\rho_j$, for $j=1,2,\ldots,\np$
	\hspace*{5mm} and a reduced dimension, $1\leq r\leq \np$.
	%\cool{!\textit{Algortihm \ref{alg:quadspq} has become superfluos. %Directly define version based on Proposition~\ref{prop:quadSPA}}!} \\
	
	\algorithmicensure~A reduced-system:  $\qdr{\bA}_r\in\mathbb{R}^{r \times r}, \, \qdr{\bB}_r \in \IR^{r \times m}, \, \qdr{\bC}_r \in \IR^{p \times r}$ and $\qdr{\bD} \in \IR^{p \times m}$.
	\begin{algorithmic} [1]   % enter the algorithmic environment
		\STATE Define reciprocal transfer function map $\TFre: s \mapsto \TF\left(\frac{1}{s} \right)$. %
		\STATE Apply Algorithm~\ref{alg:quadbt} with transfer function $\TFre$ for the given quadrature nodes to get reciprocal \ROM, i.e.,
		\begin{align*}
		\rer{A} \in \mathbb{R}^{r \times r},\quad  \rer{B}\in \mathbb{R}^{r \times m},\quad \rer{C} \in \mathbb{R}^{p \times r}, \quad \rer{D} \in \IR^{p\times m} 
		\end{align*}	
		\vspace{-0.5cm}		
		\STATE Do the reciprocal transformation on the reciprocal \ROM to get the \ROM:
		\begin{equation*} %%\label{quadbtar}
		\begin{array}{cc}
		\qdr{\bA}_r = \rer{A}^{-1} &
		\qdr{\bB}_r =   \rer{A}^{-1} \bB  \\
		\qdr{\bC}_r = - \rer{C} \rer{A}^{-1}   , \qquad & \qdr{\bD}_r = \rer{D} - \rer{C} \rer{A}^{-1} \rer{B} 
		\end{array} 
		\end{equation*}
	\end{algorithmic}
\end{algorithm}

\begin{proposition} \label{prop:quadSPA_old}
	Let $\requadU$ and $\requadL$ be as defined in 
	\eqref{eq:SpaQuad_U} and \eqref{eq:SpaQuad_L}. 
	Let 
	\begin{align*}
	\rerho_j = \rho_j/\omega_j, \qquad \text{(assuming $\omega_j\neq 0$)} \qquad \text{for } j=1,\ldots \np,
	\end{align*}	
	and let
	\begin{align*}
	\TFzer: \IC \to \IC^{p,m}, \qquad  \TFzer({s}) =  \TF(s) - \TF(0) \quad \left(= \re{C} \Kre(1/s) \re{B}  \right).
	\end{align*}
	Define the matrices $\requadLL =\requadL^*  \requadU \in \IC^{\np p \times \np m}$  and 
	$\requadMM = \requadL^* \re{A} \requadU \in \IC^{\np p \times \np m}$. Then, for $1\leq k,j\leq\np$, the $(k,j)$th block $(p,m)$ entries of matrices $\requadLL$ and $\requadMM$, respectively read as (following \Cref{def:blockMatkj}):
	\begin{align*} 
	\requadLL_{k,j} &= 
	\begin{cases} - \rerho_k \rerho_j 
	\displaystyle \frac{\TFzer(\imunit\omega_k) - \TFzer(\imunit\omega_j)}{(\imunit\omega_k)^{-1} -  (\imunit \omega_j)^{-1}} & k \neq j	\\
	{\color{red}\text{TODO correct:\,} -\rerho_k^2 \frac{d}{ds}\TFzer(s)_{s=\imunit\omega_k}} & k=j , %TODO
	\end{cases}
	\\
	\requadMM_{k,j} &= 
	\begin{cases} 
	- \rerho_k \rerho_j \displaystyle \frac{(\imunit\omega_k)^{-1} \TFzer(\imunit\omega_k) - (\imunit\omega_j)^{-1} \TFzer(\imunit\omega_j)}{(\imunit\omega_k)^{-1} -  (\imunit \omega_j)^{-1}} & k \neq j \\
	{\color{red}\text{TODO correct:\,} -\rerho_k^2 \left( \imunit\omega_k  \frac{d}{ds}\TFzer(s)_{s=\imunit\omega_k} + \imunit\TFzer(\imunit\omega_k) \right) } & k=j. %TODO
	\end{cases}
	\end{align*}
	Likewise, defining $\requadLb = \requadL^*\re{B}
	\in \IC^{\np p \times m}$ and $\requadcU^T = \re{C} \requadU\in \IC^{p \times \np m}$
	we find
	\begin{eqnarray*} 
		\requadLb_k & = & \rerho_k \TFzer(\imunit \omega_k), \ \text{for} \ 1 \leq k \leq \np,
		\\
		\requadcU_j & = &     \rerho_j \TFzer(\imunit \omega_j), \ \text{for} \ 1 \leq j \leq \np.
	\end{eqnarray*}
\end{proposition}
